# Supplementary material for: Algebraic theory of endohedrally confined diatomic molecules: application to H$_2$@C$_{60}$
Source: arXiv:1605.00145 source file (2016-08-11)
Supplement: Supplementary file 1 [file supplementary_PRA.pdf]

# Supplementary Material:
# Algebraic theory of endohedrally confined diatomic molecules: application to $H_2@C_{60}$

Lorenzo Fortunato
*Dipartimento di Fisica e Astronomia "G.Galilei", Università di Padova and I.N.F.N.- Sez. di Padova; v. Marzolo, 8, I-35131, Padova, ITALY*

Francisco Pérez-Bernal
*Grupo de investigación en Física Molecular, Atómica y Nuclear (GIFMAN-UHU), Unidad Asociada al CSIC. Depto. de Ciencias Integradas, Universidad de Huelva, 21071 Huelva, SPAIN*

We provide in Tab. I the present supplemental material calculated levels using finer fit $F_1$ parameters given in Tab. III of the main text. The included levels have $v$ = 0,1 and 2 vibrational quanta, $N_q \leq 4$, and $\Lambda \leq 5$. In addition to the term energy, expressed in cm$^{-1}$ units, $|C_{vJN_qL\Lambda}|^2$ is also included, the maximum squared coefficient of the corresponding eigenstate expressed in the algebraic basis

$$\begin{array}{ccccccccc} u_p(4) \oplus u_q(3) & \supset & so_p(4) \oplus u_q(3) & \supset & so_p(3) \oplus so_q(3) & \supset & so_{pq}(3 \\ N_p \quad\quad N_q & & \omega & & J \quad\quad\quad L & & \Lambda \end{array} , \qquad (1)$$

taking into account hat $\omega$ is related to $v$ quantum number through $v = \frac{1}{2}(N_p - \omega)$

TABLE I: Calculated energy levels for $H_2@C_{60}$ with $v = 0, 1, 2$ using finer fit $F_1$ parameters (See Tab. III main text). States are denoted by the quantum numbers $vJN_qL\Lambda$. Term energy values are expressed in cm$^{-1}$. $|C_{vJN_qL\Lambda}|^2$ is the value of the eigenstate maximum squared component in basis $|N_pvJ; N_qL; \Lambda\rangle$, used to assign $vJN_qL\Lambda$ quantum numbers.

| $vJN_qL\Lambda$ | Calc. | $\|C_{vJN_qL\Lambda}\|^2$ | $vJN_qL\Lambda$ | Calc. | $\|C_{vJN_qL\Lambda}\|^2$ | $vJN_qL\Lambda$ | Calc. | $\|C_{vJN_qL\Lambda}\|^2$ |
|---|---|---|---|---|---|---|---|---|
| 00000 | 0.000 00 | 1.000 00 | 12002 | 4402.634 63 | 1.000 00 | 20200 | 8295.760 73 | 0.996 60 |
| 01001 | 116.440 50 | 1.000 00 | 10222 | 4452.279 21 | 0.998 76 | 21222 | 8373.319 53 | 0.999 79 |
| 00111 | 180.904 84 | 0.999 58 | 10200 | 4470.960 66 | 0.997 46 | 21221 | 8383.826 58 | 0.698 58 |
| 01111 | 292.330 15 | 1.000 00 | 11222 | 4554.856 04 | 0.999 85 | 21223 | 8384.568 52 | 0.999 36 |
| 01112 | 298.430 44 | 0.999 83 | 11221 | 4564.888 96 | 0.730 56 | 22112 | 8385.399 91 | 1.000 00 |
| 01110 | 307.825 16 | 1.000 00 | 11223 | 4565.097 80 | 0.999 52 | 22113 | 8393.514 77 | 0.999 83 |
| 02002 | 348.564 21 | 1.000 00 | 12112 | 4581.709 08 | 1.000 00 | 22111 | 8398.458 57 | 0.999 21 |
| 00222 | 372.355 78 | 0.999 11 | 11201 | 4588.080 09 | 0.730 07 | 21201 | 8408.494 23 | 0.697 93 |
| 00200 | 391.134 06 | 0.998 17 | 12113 | 4589.087 63 | 0.999 88 | 18335 | 8483.255 43 | 0.999 90 |
| 01222 | 481.823 42 | 0.999 89 | 12111 | 4593.529 83 | 0.999 41 | 20333 | 8486.475 28 | 0.997 37 |
| 01223 | 490.983 32 | 0.999 66 | 08335 | 4617.626 85 | 0.999 93 | 23003 | 8514.175 07 | 1.000 00 |
| 01221 | 491.281 20 | 0.767 51 | 10333 | 4658.044 02 | 0.998 03 | 20311 | 8517.445 92 | 0.994 59 |
| 01201 | 513.031 38 | 0.767 14 | 10311 | 4689.190 83 | 0.995 94 | 21333 | 8580.256 29 | 0.999 55 |
| 02112 | 524.437 01 | 1.000 00 | 13003 | 4730.633 86 | 1.000 00 | 22223 | 8583.434 21 | 0.999 86 |
| 02113 | 531.028 31 | 0.999 91 | 11333 | 4758.462 84 | 0.999 67 | 22222 | 8584.590 66 | 0.867 59 |
| 02111 | 534.950 51 | 0.999 58 | 11332 | 4772.093 76 | 0.852 14 | 22224 | 8594.269 73 | 0.999 67 |
| 00333 | 574.351 56 | 0.998 58 | 11334 | 4772.134 77 | 0.999 27 | 21332 | 8594.778 55 | 0.829 15 |
| 00311 | 605.655 65 | 0.997 07 | 12223 | 4776.256 65 | 0.999 90 | 21334 | 8595.275 70 | 0.999 02 |
| 01333 | 681.873 36 | 0.999 76 | 12222 | 4777.493 21 | 0.882 63 | 22221 | 8597.255 69 | 1.000 00 |
| 01334 | 694.098 81 | 0.999 48 | 12224 | 4786.107 04 | 0.999 75 | 22220 | 8604.700 41 | 0.996 60 |
| 01332 | 694.477 68 | 0.876 70 | 12221 | 4788.788 56 | 1.000 00 | 21311 | 8611.841 79 | 0.999 11 |
| 03003 | 694.856 57 | 1.000 00 | 11311 | 4790.093 78 | 0.999 34 | 22202 | 8613.724 71 | 0.867 24 |
| 01311 | 713.544 83 | 0.999 53 | 12220 | 4795.418 82 | 0.997 46 | 21312 | 8631.672 23 | 0.827 93 |
| 02223 | 715.261 66 | 0.999 93 | 12202 | 4805.266 68 | 0.882 40 | 21310 | 8646.008 80 | 0.998 50 |
| 02222 | 716.559 54 | 0.899 04 | 11312 | 4807.666 54 | 0.851 23 | 23113 | 8696.209 56 | 1.000 00 |
| 02224 | 724.059 39 | 0.999 82 | 11310 | 4821.154 34 | 0.998 90 | 18445 | 8697.387 67 | 0.999 90 |

Continued on next page

**TABLE I – continued from previous page**

| $vJN_qL\Lambda$ | Calc. | $\lvert C_{vJN_qL\Lambda}\rvert^2$ | $vJN_qL\Lambda$ | Calc. | $\lvert C_{vJN_qL\Lambda}\rvert^2$ | $vJN_qL\Lambda$ | Calc. | $\lvert C_{vJN_qL\Lambda}\rvert^2$ |
|---|---|---|---|---|---|---|---|---|
| 02221 | 726.425 42 | 1.000 00 | 08445 | 4828.207 81 | 0.999 93 | 18444 | 8703.590 77 | 0.999 87 |
| 01312 | 728.784 35 | 0.876 04 | 08444 | 4833.700 55 | 0.999 91 | 23114 | 8704.709 50 | 0.999 90 |
| 02220 | 732.228 06 | 0.998 17 | 10444 | 4874.344 49 | 0.997 21 | 20444 | 8706.288 87 | 0.996 28 |
| 01310 | 741.282 34 | 0.999 22 | 13113 | 4909.676 44 | 1.000 00 | 23112 | 8707.971 05 | 0.999 68 |
| 02202 | 742.950 98 | 0.898 89 | 13114 | 4917.395 16 | 0.999 92 | 20422 | 8749.667 05 | 0.992 50 |
| 00444 | 786.891 06 | 0.997 99 | 10422 | 4917.962 68 | 0.994 36 | 20400 | 8768.274 36 | 0.991 05 |
| 00422 | 830.724 59 | 0.995 91 | 13112 | 4920.323 25 | 0.999 76 | 22334 | 8792.026 41 | 0.999 71 |
| 00400 | 849.518 54 | 0.995 09 | 10400 | 4936.668 07 | 0.993 25 | 22333 | 8792.054 00 | 0.937 57 |
| 03113 | 870.704 09 | 1.000 00 | 11444 | 4972.622 38 | 0.999 46 | 21444 | 8797.741 51 | 0.999 28 |
| 03114 | 877.591 46 | 0.999 95 | 12334 | 4981.364 40 | 0.999 79 | 22332 | 8800.436 99 | 0.859 24 |
| 03112 | 880.174 56 | 0.999 83 | 12333 | 4981.498 25 | 0.945 74 | 22335 | 8805.590 27 | 0.999 50 |
| 01444 | 892.479 91 | 0.999 61 | 12332 | 4989.342 20 | 0.888 22 | 22331 | 8813.966 82 | 0.978 85 |
| 01445 | 907.776 61 | 0.999 29 | 11445 | 4989.731 94 | 0.999 01 | 21443 | 8816.236 73 | 0.882 12 |
| 01443 | 908.237 54 | 0.917 37 | 11443 | 4989.829 04 | 0.899 46 | 21445 | 8816.540 77 | 0.998 67 |
| 02334 | 916.648 61 | 0.999 85 | 12335 | 4993.692 67 | 0.999 63 | 22312 | 8823.798 74 | 0.858 91 |
| 02333 | 916.884 34 | 0.954 23 | 12331 | 5001.216 65 | 0.983 58 | 22313 | 8838.235 64 | 0.937 25 |
| 02332 | 924.076 01 | 0.915 43 | 12312 | 5012.777 20 | 0.887 98 | 21422 | 8841.965 38 | 0.998 68 |
| 02335 | 927.657 33 | 0.999 73 | 11422 | 5016.908 51 | 0.999 01 | 22311 | 8844.732 25 | 0.978 13 |
| 02331 | 934.296 51 | 0.987 71 | 12313 | 5026.047 19 | 0.945 52 | 21421 | 8853.287 92 | 0.563 12 |
| 01422 | 936.821 75 | 0.999 29 | 11421 | 5027.934 16 | 0.588 14 | 21423 | 8865.460 97 | 0.880 40 |
| 01421 | 947.472 03 | 0.619 83 | 12311 | 5031.997 17 | 0.983 09 | 21401 | 8891.275 56 | 0.562 43 |
| 02312 | 947.773 98 | 0.915 26 | 11423 | 5037.843 72 | 0.898 17 | 23223 | 8893.780 66 | 0.889 39 |
| 01423 | 955.099 11 | 0.916 44 | 11401 | 5062.764 83 | 0.587 63 | 23224 | 8895.174 95 | 0.999 91 |
| 02313 | 959.744 87 | 0.954 09 | 13223 | 5103.968 61 | 0.901 53 | 23222 | 8904.385 92 | 0.999 79 |
| 02311 | 965.119 87 | 0.987 39 | 13224 | 5105.066 68 | 0.999 93 | 23225 | 8905.811 88 | 0.999 79 |
| 01401 | 979.032 19 | 0.619 46 | 13222 | 5113.398 03 | 0.999 85 | 23221 | 8912.402 82 | 0.999 21 |
| 03223 | 1061.472 68 | 0.914 84 | 13225 | 5114.724 56 | 0.999 85 | 23203 | 8924.115 21 | 0.889 09 |
| 03224 | 1062.278 22 | 0.999 95 | 13221 | 5120.633 81 | 0.999 42 | 24004 | 8925.106 97 | 1.000 00 |
| 03222 | 1069.682 95 | 0.999 89 | 13203 | 5132.886 30 | 0.901 32 | 22444 | 9010.348 19 | 0.959 19 |
| 03225 | 1070.894 65 | 0.999 89 | 14004 | 5164.432 18 | 1.000 00 | 22445 | 9011.176 37 | 0.999 55 |
| 03221 | 1076.100 88 | 0.999 58 | 12444 | 5196.336 44 | 0.965 02 | 22443 | 9018.868 21 | 0.916 49 |
| 03203 | 1088.941 67 | 0.914 70 | 12445 | 5197.032 25 | 0.999 66 | 22442 | 9034.042 82 | 0.907 87 |
| 02444 | 1128.043 62 | 0.970 89 | 12443 | 5204.288 50 | 0.932 43 | 22422 | 9054.263 28 | 0.691 38 |
| 02445 | 1128.597 77 | 0.999 76 | 12442 | 5217.981 12 | 0.938 31 | 22423 | 9056.393 20 | 0.915 96 |
| 02443 | 1135.325 58 | 0.947 56 | 12422 | 5240.277 83 | 0.736 70 | 22424 | 9073.081 11 | 0.959 19 |
| 02442 | 1147.407 02 | 0.960 06 | 12423 | 5241.891 35 | 0.932 04 | 22421 | 9074.730 29 | 0.999 25 |
| 04004 | 1153.045 72 | 1.000 00 | 12424 | 5257.153 91 | 0.965 03 | 22420 | 9087.519 23 | 0.990 12 |
| 02422 | 1172.112 44 | 0.777 55 | 12421 | 5258.848 65 | 0.999 45 | 22402 | 9093.124 25 | 0.768 94 |
| 02423 | 1173.146 47 | 0.947 28 | 12420 | 5270.135 24 | 0.992 57 | 23334 | 9101.521 36 | 0.952 95 |
| 02424 | 1186.858 42 | 0.970 91 | 12402 | 5276.793 54 | 0.789 06 | 23335 | 9104.703 40 | 0.999 81 |
| 02421 | 1188.559 03 | 0.999 61 | 13334 | 5308.235 38 | 0.958 83 | 23333 | 9105.789 71 | 0.891 42 |
| 02420 | 1198.342 75 | 0.994 62 | 13335 | 5311.021 19 | 0.999 86 | 24114 | 9107.088 44 | 1.000 00 |
| 02402 | 1206.112 54 | 0.811 70 | 13333 | 5312.261 85 | 0.910 96 | 23332 | 9115.681 54 | 0.979 46 |
| 03334 | 1262.039 47 | 0.965 02 | 13332 | 5320.992 80 | 0.982 79 | 24115 | 9115.874 02 | 0.999 93 |
| 03335 | 1264.417 74 | 0.999 90 | 13331 | 5327.869 74 | 0.999 34 | 24113 | 9118.342 70 | 0.999 83 |
| 03333 | 1265.764 69 | 0.929 97 | 13330 | 5331.578 79 | 0.998 90 | 23331 | 9123.360 70 | 0.999 11 |
| 03332 | 1273.321 43 | 0.986 06 | 13313 | 5340.712 48 | 0.911 02 | 23330 | 9127.489 92 | 0.998 50 |
| 03331 | 1279.368 71 | 0.999 52 | 14114 | 5343.432 26 | 1.000 00 | 23313 | 9134.507 83 | 0.891 48 |
| 03330 | 1282.644 05 | 0.999 22 | 14115 | 5351.399 82 | 0.999 95 | 23314 | 9149.118 74 | 0.952 48 |
| 03313 | 1294.058 74 | 0.930 02 | 14113 | 5353.615 44 | 0.999 88 | 23312 | 9153.383 45 | 0.978 44 |
| 03314 | 1306.132 80 | 0.964 78 | 13314 | 5354.112 79 | 0.958 49 | 24224 | 9304.028 86 | 0.896 03 |
| 03312 | 1309.660 34 | 0.985 53 | 13312 | 5358.019 22 | 0.982 04 | 24225 | 9306.658 15 | 0.999 93 |
| 04114 | 1328.859 54 | 1.000 00 | 13445 | 5523.381 84 | 0.975 53 | 24223 | 9313.658 21 | 0.999 86 |
| 04115 | 1335.960 87 | 0.999 96 | 13444 | 5526.215 02 | 0.947 97 | 23445 | 9320.137 65 | 0.971 73 |
| 04113 | 1337.914 75 | 0.999 91 | 13443 | 5533.690 50 | 0.949 34 | 24222 | 9322.168 72 | 0.999 63 |
| 03445 | 1473.487 41 | 0.979 43 | 14224 | 5537.149 44 | 0.907 30 | 23444 | 9323.131 30 | 0.937 37 |
| 03444 | 1476.120 41 | 0.958 35 | 14225 | 5539.368 01 | 0.999 95 | 23443 | 9331.364 39 | 0.934 39 |
| 03443 | 1482.772 85 | 0.962 37 | 13442 | 5542.533 35 | 0.985 37 | 24204 | 9334.914 27 | 0.895 82 |
| 03442 | 1490.481 68 | 0.988 83 | 14223 | 5545.692 00 | 0.999 90 | 23442 | 9341.330 93 | 0.981 53 |
| 03441 | 1496.536 83 | 0.997 87 | 13441 | 5549.439 80 | 0.997 14 | 23441 | 9349.071 40 | 0.996 29 |
| 03423 | 1516.883 48 | 0.806 39 | 14222 | 5553.384 36 | 0.999 72 | 23423 | 9363.203 19 | 0.747 44 |

Continued on next page

**TABLE I – continued from previous page**

| $vJN_qL\Lambda$ | Calc. | $\|C_{vJN_qL\Lambda}\|^2$ | $vJN_qL\Lambda$ | Calc. | $\|C_{vJN_qL\Lambda}\|^2$ | $vJN_qL\Lambda$ | Calc. | $\|C_{vJN_qL\Lambda}\|^2$ |
|---|---|---|---|---|---|---|---|---|
| 04224 | 1519.111 31 | 0.919 67 | 14204 | 5566.573 18 | 0.907 14 | 23424 | 9368.471 69 | 0.937 48 |
| 03424 | 1520.517 11 | 0.958 43 | 13423 | 5566.586 21 | 0.776 50 | 23422 | 9380.710 37 | 0.981 34 |
| 04225 | 1520.917 75 | 0.999 97 | 13424 | 5571.054 11 | 0.948 07 | 23425 | 9384.387 10 | 0.971 17 |
| 04223 | 1526.532 21 | 0.999 93 | 13422 | 5582.297 49 | 0.985 25 | 23421 | 9392.970 18 | 0.995 25 |
| 03422 | 1530.678 84 | 0.988 75 | 13425 | 5585.599 39 | 0.975 11 | 23403 | 9402.841 94 | 0.805 05 |
| 04222 | 1533.365 36 | 0.999 80 | 13421 | 5593.392 26 | 0.996 37 | 25005 | 9433.092 23 | 1.000 00 |
| 03425 | 1533.582 13 | 0.979 14 | 13403 | 5603.843 02 | 0.821 49 | 24335 | 9512.271 47 | 0.958 31 |
| 03421 | 1540.547 41 | 0.997 31 | 15005 | 5701.000 45 | 1.000 00 | 24334 | 9514.535 77 | 0.899 97 |
| 04204 | 1547.041 33 | 0.919 56 | 14335 | 5741.871 71 | 0.963 47 | 24333 | 9523.036 39 | 0.977 68 |
| 03403 | 1551.634 55 | 0.840 22 | 14334 | 5744.070 13 | 0.917 14 | 24332 | 9530.862 68 | 0.999 62 |
| 04335 | 1720.083 88 | 0.968 90 | 14333 | 5751.558 06 | 0.980 99 | 24331 | 9536.586 57 | 0.999 37 |
| 05005 | 1720.102 55 | 1.000 00 | 14332 | 5758.572 60 | 0.999 72 | 24314 | 9545.360 12 | 0.900 00 |
| 04334 | 1722.173 69 | 0.934 03 | 14331 | 5763.739 98 | 0.999 54 | 24315 | 9560.227 96 | 0.957 96 |
| 04333 | 1728.640 57 | 0.984 32 | 14314 | 5774.458 92 | 0.917 16 | 24313 | 9563.450 22 | 0.977 11 |
| 04332 | 1734.813 38 | 0.999 80 | 14315 | 5788.080 27 | 0.963 21 | 19445 | 9605.707 71 | 0.999 89 |
| 04331 | 1739.398 25 | 0.999 67 | 09445 | 5790.692 36 | 0.999 93 | 25115 | 9615.007 42 | 1.000 00 |
| 04314 | 1752.217 75 | 0.934 05 | 14313 | 5791.031 15 | 0.980 57 | 25114 | 9626.035 32 | 0.999 90 |
| 04315 | 1764.482 75 | 0.968 72 | 15115 | 5879.947 42 | 1.000 00 | 24445 | 9731.914 03 | 0.944 80 |
| 04313 | 1767.146 42 | 0.984 02 | 15114 | 5889.917 69 | 0.999 92 | 24444 | 9737.451 53 | 0.936 79 |
| 05115 | 1895.874 24 | 1.000 00 | 14445 | 5958.056 86 | 0.953 76 | 24443 | 9745.681 37 | 0.976 58 |
| 05114 | 1904.734 36 | 0.999 95 | 14444 | 5963.099 41 | 0.949 86 | 24442 | 9753.196 92 | 0.994 81 |
| 04445 | 1932.557 76 | 0.962 62 | 14443 | 5970.399 00 | 0.980 91 | 24441 | 9758.708 60 | 0.999 25 |
| 04444 | 1937.058 99 | 0.961 69 | 14442 | 5977.122 30 | 0.995 75 | 24440 | 9761.598 23 | 0.999 07 |
| 04443 | 1943.419 17 | 0.984 98 | 14441 | 5982.078 67 | 0.999 44 | 24424 | 9773.397 19 | 0.760 25 |
| 04442 | 1949.326 64 | 0.996 63 | 14440 | 5984.683 62 | 0.999 32 | 24425 | 9780.160 61 | 0.944 82 |
| 04441 | 1953.706 05 | 0.999 61 | 14424 | 5999.715 84 | 0.786 70 | 24423 | 9789.434 73 | 0.976 32 |
| 04440 | 1956.014 23 | 0.999 52 | 14425 | 6005.558 89 | 0.953 78 | 24422 | 9802.144 21 | 0.993 96 |
| 04424 | 1974.467 05 | 0.814 43 | 14423 | 6014.063 73 | 0.980 72 | 25225 | 9811.612 57 | 0.898 44 |
| 04425 | 1979.353 61 | 0.962 64 | 14422 | 6025.608 11 | 0.995 12 | 24404 | 9813.437 41 | 0.816 48 |
| 04423 | 1987.028 18 | 0.984 85 | 14404 | 6037.355 40 | 0.831 78 | 25224 | 9820.698 76 | 0.999 91 |
| 04422 | 1997.336 74 | 0.996 19 | 15225 | 6073.363 50 | 0.909 41 | 25223 | 9829.557 05 | 0.999 78 |
| 04404 | 2009.589 67 | 0.849 26 | 15224 | 6081.406 74 | 0.999 93 | 25205 | 9842.866 62 | 0.898 29 |
| 05225 | 2085.859 01 | 0.921 44 | 15223 | 6089.411 51 | 0.999 84 | 25335 | 10 021.368 07 | 0.902 78 |
| 05224 | 2092.831 00 | 0.999 95 | 15205 | 6103.111 70 | 0.909 30 | 25334 | 10 029.066 33 | 0.976 26 |
| 05223 | 2099.940 94 | 0.999 88 | 15335 | 6279.603 10 | 0.919 14 | 25333 | 10 036.986 15 | 0.999 78 |
| 05205 | 2114.073 02 | 0.921 37 | 15334 | 6286.364 71 | 0.979 64 | 25332 | 10 043.657 80 | 0.999 64 |
| 05335 | 2288.315 39 | 0.935 31 | 15333 | 6293.456 54 | 0.999 84 | 25315 | 10 053.271 05 | 0.902 78 |
| 05334 | 2294.137 94 | 0.983 08 | 15332 | 6299.482 17 | 0.999 74 | 25314 | 10 071.013 90 | 0.975 89 |
| 05333 | 2300.373 21 | 0.999 88 | 15315 | 6310.970 40 | 0.919 15 | 26115 | 10 227.120 72 | 0.999 93 |
| 05332 | 2305.722 47 | 0.999 81 | 15314 | 6327.209 79 | 0.979 37 | 25445 | 10 242.992 72 | 0.936 93 |
| 05315 | 2319.232 28 | 0.935 32 | 15445 | 6497.469 17 | 0.949 48 | 25444 | 10 250.220 91 | 0.973 44 |
| 05314 | 2333.849 86 | 0.982 89 | 15444 | 6503.865 94 | 0.978 11 | 25443 | 10 257.609 60 | 0.993 35 |
| 05445 | 2502.172 50 | 0.961 00 | 15443 | 6510.467 35 | 0.994 46 | 25442 | 10 263.870 88 | 0.999 61 |
| 05444 | 2507.733 86 | 0.982 59 | 15442 | 6516.097 68 | 0.999 71 | 25441 | 10 268.337 95 | 0.999 49 |
| 05443 | 2513.526 73 | 0.995 53 | 15441 | 6520.129 94 | 0.999 63 | 25425 | 10 280.935 66 | 0.764 47 |
| 05442 | 2518.501 45 | 0.999 80 | 16115 | 6525.316 00 | 0.999 95 | 25424 | 10 296.179 51 | 0.973 25 |
| 05441 | 2522.079 12 | 0.999 74 | 15425 | 6535.886 55 | 0.790 13 | 25423 | 10 309.278 22 | 0.992 79 |
| 05425 | 2541.171 11 | 0.817 16 | 15424 | 6549.492 55 | 0.977 98 | 25405 | 10 321.326 64 | 0.820 97 |
| 05424 | 2553.055 38 | 0.982 49 | 15423 | 6561.398 82 | 0.994 05 | 26225 | 10 421.332 89 | 0.999 93 |
| 05423 | 2563.696 51 | 0.995 24 | 15405 | 6573.837 49 | 0.835 84 | 26224 | 10 430.471 29 | 0.999 85 |
| 05405 | 2576.573 24 | 0.852 82 | 16225 | 6716.402 14 | 0.999 95 | 26335 | 10 629.067 47 | 0.975 04 |
| 06115 | 2576.734 14 | 0.999 96 | 16224 | 6724.652 92 | 0.999 89 | 26334 | 10 637.068 26 | 0.999 85 |
| 06225 | 2764.476 40 | 0.999 97 | 16335 | 6920.794 86 | 0.978 53 | 26333 | 10 644.396 29 | 0.999 76 |
| 06224 | 2771.799 89 | 0.999 92 | 16334 | 6927.948 64 | 0.999 89 | 26315 | 10 672.051 44 | 0.974 78 |
| 06335 | 2965.287 27 | 0.982 10 | 16333 | 6934.563 12 | 0.999 83 | 26445 | 10 849.338 67 | 0.971 06 |
| 06334 | 2971.568 45 | 0.999 92 | 16315 | 6962.556 36 | 0.978 35 | 26444 | 10 856.636 80 | 0.992 22 |
| 06333 | 2977.437 93 | 0.999 88 | 16445 | 7137.504 53 | 0.976 04 | 26443 | 10 863.386 58 | 0.999 75 |
| 06315 | 3005.796 60 | 0.981 97 | 16444 | 7144.012 35 | 0.993 47 | 26442 | 10 868.895 86 | 0.999 67 |
| 06445 | 3178.186 32 | 0.980 84 | 16443 | 7150.075 27 | 0.999 82 | 26425 | 10 896.636 69 | 0.970 92 |
| 06444 | 3183.886 45 | 0.994 69 | 16442 | 7155.046 71 | 0.999 76 | 26424 | 10 910.075 00 | 0.991 82 |
| 06443 | 3189.238 08 | 0.999 87 | 16425 | 7184.314 13 | 0.975 94 | 27225 | 11 120.252 81 | 0.999 89 |

Continued on next page

**TABLE I – continued from previous page**

| $vJN_qL\Lambda$ | Calc. | $\|C_{vJN_qL\Lambda}\|^2$ | $vJN_qL\Lambda$ | Calc. | $\|C_{vJN_qL\Lambda}\|^2$ | $vJN_qL\Lambda$ | Calc. | $\|C_{vJN_qL\Lambda}\|^2$ |
|---|---|---|---|---|---|---|---|---|
| 06442 | 3193.648 32 | 0.999 83 | 16424 | 7196.525 40 | 0.993 17 | 27335 | 11 326.242 64 | 0.999 89 |
| 06425 | 3224.533 66 | 0.980 77 | 17225 | 7454.462 19 | 0.999 92 | 27334 | 11 334.077 78 | 0.999 83 |
| 06424 | 3235.446 25 | 0.994 48 | 17335 | 7657.214 28 | 0.999 92 | 27445 | 11 545.084 18 | 0.991 29 |
| 07225 | 3544.308 33 | 0.999 94 | 17334 | 7664.278 80 | 0.999 88 | 27444 | 11 552.197 79 | 0.999 82 |
| 07335 | 3743.597 66 | 0.999 94 | 17445 | 7872.628 08 | 0.992 66 | 27443 | 11 558.475 16 | 0.999 76 |
| 07334 | 3749.860 97 | 0.999 91 | 17444 | 7879.007 99 | 0.999 87 | 27425 | 11 599.811 57 | 0.990 98 |
| 07445 | 3955.344 46 | 0.994 01 | 17443 | 7884.667 13 | 0.999 83 | 28335 | 12 107.319 57 | 0.999 87 |
| 07444 | 3960.968 19 | 0.999 91 | 20000 | 7890.204 38 | 1.000 00 | 28445 | 12 324.772 97 | 0.999 86 |
| 07443 | 3965.984 73 | 0.999 88 | 17425 | 7926.284 11 | 0.992 44 | 28444 | 12 331.662 82 | 0.999 82 |
| 07425 | 4007.901 75 | 0.993 85 | 21001 | 7994.830 56 | 1.000 00 | 29445 | 13 182.342 47 | 0.999 85 |
| 10000 | 4072.363 55 | 1.000 00 | 20111 | 8078.430 42 | 0.999 21 | | | |
| 11001 | 4182.706 34 | 1.000 00 | 21111 | 8176.931 34 | 1.000 00 | | | |
| 10111 | 4257.051 75 | 0.999 41 | 21112 | 8184.419 90 | 0.999 68 | | | |
| 11111 | 4361.802 04 | 1.000 00 | 21110 | 8196.062 31 | 1.000 00 | | | |
| 11112 | 4368.621 49 | 0.999 76 | 22002 | 8203.325 65 | 1.000 00 | | | |
| 11110 | 4379.172 83 | 1.000 00 | 20222 | 8277.188 32 | 0.998 34 | | | |
